# Supplementary material for: Automated Detection of GDPR Disclosure Requirements in Privacy Policies using Deep Active Learning
Source: arXiv:2111.04224 source file (2021-11-08)
Supplement: Supplementary file 1 [file appendix.tex]

% \clearpage
% \begin{appendices}
% \section{GDPR Privacy Disclosure Requirements}~\label{appendix:categories}
% In the following, we describe the 18 categories of GDPR requirements~\cite{gdpr_legislation} for the privacy policies that are identified by two legal experts. More details about these requirements can be found in GDPR regulation (Chapter 3, Art. 12--23)~\cite{gdpr}.

% \textbf{(1) Data Categories}: No matter whether data is collected from users or any other sources, privacy policies should provide the information about the categories of personal data collected, stored or processed by any organization or third parties.% For example, \textit{Apple} discloses certain categories of personal information they collect as following - \textit{``We may collect a variety of information, including your name, mailing address, phone number, email address, contact preferences, device identifiers, IP address, location information, credit card information and profile information where the contact is via social media.'' }

% \textbf{(2) Processing Purpose}: Privacy policy should include the purposes of processing user's personal data as well as lawful basis to process those data. Before any organization begin to process user's data, they must determine their lawful basis, which in most cases require that the data processing is \textit{necessary} for specific purposes.% For example, \textit{Apple} describes one of the purposes for collecting users' personal information as following - \textit{``We also use personal information to help us create, develop, operate, deliver, and improve our products, services, content and advertising, and for loss prevention and anti-fraud purposes.''}

% \textbf{(3) Data Recipients}: An organization should disclose the information about the recipients to whom users' personal data have been or will be shared, including the recipients from third countries or international organizations. For example, \textit{Msn.com} provides the information regarding recipients of user's personal data as following - \textit{``We may share your personal information with third parties, such as advertisers, sponsors, and other promotional and business partners.''}

% \textbf{(4) Source of Data}: Privacy policy should mention information about which source personal data originate from if they are not obtained directly from users. For example, \textit{TheGuardian.com} discloses the source of some personal information as following - \textit{``We may obtain information about you from partners so that we can make our online advertising more relevant.''}

% \textbf{(5) Provision Requirement}: Privacy policy should include whether providing personal data is required, or if the user is obligated to provide the personal data and consequences for not doing so. For example, \textit{Gettyimages.com} discloses the existence of this right in their privacy policy as following - \textit{``You may always choose not to provide personal data, but if you so choose, certain products and services may not be available to you.''}

% \textbf{(6) Data Safeguards}: If the controller intends to transfer data to a third country or an international organization with the absence of an adequacy decision, reference of appropriate safeguards of personal data should be provided in the privacy policy. Additionally, privacy policy also needs to provide the means to obtain a copy of the available safeguards to protect users' personal data. %For example, \textit{The Guardian} discloses this requirement in their privacy policy as following - \textit{``Whenever we transfer your personal data out of the European Economic Area (EEA), we ensure similar protection and put in place at least one of these safeguards ...''}

% \textbf{(7) Profiling}: GDPR has provisions on profiling or other automated-decision making. Automated decision making is defined as making a decision solely by automated means without any human involvement, and profiling, which can be a part of automated-decision making, is defined as automated processing of personal data to evaluate certain things about an individual. According to (Art. 22) of GDPR, data controllers can carry out such decision-making if they have a lawful basis and explicit consent of users for the relevant processing of personal data. The privacy policy should include the existence of any automated-decision making, including profiling and what information is used for such decision-making.% For example, \textit{Dropbox} discloses information regarding profiling as following - \textit{``Dropbox collects and processes your personal information using automated decision-making (including machine learning) to provide, improve, and market the dropbox services in furtherance of its legitimate interests or based on your consent when appropriate.''}

% \textbf{(8) Storage Period}: Privacy policy should disclose the period for which personal data will be stored, or if not possible, the criteria used to determine that period. GDPR mandates that personal data shall not be kept longer than is necessary for the purposes for which it is processed. Period of personal data stored by a data controller should be limited to a strict minimum and a time limit for the deletion of the data should be determined and disclosed in the privacy policy by the data controller. %For instance, \textit{Academia.edu} discloses the personal data storage period in the following manner - \textit{``academia.edu retains the personal information we receive as described in this privacy policy for as long as you use the academia.edu service or as necessary to fulfill the purpose(s) for which it was collected.''}

% \textbf{(9) Adequacy Decision}: When controllers intend to transfer personal data to a third country or international organization, the existence of absence of an adequacy decision by the European Commission must be disclosed in the privacy policy. Adequacy decision made by the EU Commission is based on whether a country outside of EU offers an adequate level of data protection. For example, Oracle discloses this requirement as following - \textit{``If personal information is transferred to an oracle recipient in a country that does not provide an adequate level of protection for personal information, oracle will take measures designed to adequately protect information about you, such as ensuring that such transfers are subject to the terms of the EU model clauses.''}

% \textbf{(10) Controller's Contact}: Data controllers shall provide their identity and contact details along with the contact details of any controller's representative, if applicable. %For example, \textit{The Guardian} news provides the data controller's contact information as following - \textit{``The data controller for our sites and apps is Guardian News \& Media Limited, Kings Place, 90 York Way, London N1 9GU.4''}.
    
% \textbf{(11) DPO Contact}: Every organization that collects and process the personal information of EU citizens have to appoint a Data Protection Officer (DPO) and contact information of the DPO has to be provided in the privacy policy. %For example, \textit{Microsoft} provides the information about their Data Protection Officer as following - \textit{``If you have a privacy concern, complaint, or question for the Microsoft Chief Privacy Officer or EU Data Protection Officer, please contact us by using our web form.''}
    
% \textbf{(12) Withdraw Consent}: Privacy policy should include the existence of users' right to withdraw consent at any time. For example, \textit{Nextdoor.com} discloses the existence of this right as following - \textit{``If you wish, you can access the content of the (electronic) consent as well as revoke the consent with effect for the future at any time.''}
    
% \textbf{(13) Lodge Complaint}: Privacy policy should include the existence of users' right to lodge a complaint with a supervisory authority. For example, \textit{Gofundme.com} discloses the existence of this right in their privacy policy as following - \textit{``You also have the right to lodge a complaint with the local data protection authority if you believe that we have not complied with applicable data protection laws.''} 
    

% \textbf{(14) Right to Access}: Data controller should disclose the existence of users' right to request the controller to access or rectify the personal data. According to GDPR (Art. 15), users have right to obtain information about whether their personal data is being collected, used or stored; the categories of the data; with whom the data have been or will be disclosed; whether the data has been or will be transferred to a third country or organization; and how long the data will be stored or processed. For example, legacy.com discloses that \textit{``you may access the information we hold about you anytime via your profile/account.''}
    
% \textbf{(15) Right to Erase}: Data controller must disclose the existence of users' right to erase personal data. As mentioned in GDPR (Art. 17), an organization shall have an obligation to erase personal data when data are no longer necessary for the purposes they were collected or stored. In addition to that, if users withdraw their consent any time, corresponding personal data must be erased. %For example, \textit{Ranker.com} describes this right as following - \textit{``If you no longer want us to use your information during the provision of the Services to you, you can request that we erase your personal information and close your Account.''}
    
% \textbf{(16) Right to Restrict}: Privacy policy should include the existence of user's right to restrict or suppress the processing of their personal data. For example, \textit{Politico.com} discloses this right as following - \textit{"You may also have rights to restrict our processing of your personal data"}
    
% \textbf{(17) Right to Object}: Privacy policy should include the existence of user's right to object the processing of their personal data. For example, users have the absolute right to stop their data being used in direct marketing.% \textit{Ranker.com} discloses the existence of users' right to object as following - \textit{``If you object to such processing we will no longer process your personal information for these purposes.''}
    
% \textbf{(18) Right to Data Portability}: Privacy policy should include the existence of users' right to receive the personal data in a structured, commonly used and machine-readable format, and right to transfer those data to another data controller. %For example, \textit{Oclc.org} discloses this right as following - \textit{``You may receive personal data that you have provided to us in a structured, commonly used and machine-readable format and have the right to transmit it to other data controllers.''}

% \section{Interface of Policy Annotation Tool}~\label{appendix:tool-interface}
% We build an annotation tool for our annotators which allows the annotators to annotate one segment at a time. For each segment, there are 18 available labels corresponding the GDPR requirements. We also provide an additional \textit{Other} option to annotate segments that do not represent any of the 18 requirements.
% \begin{figure}[!ht]
% \centering
% \includegraphics[width=\linewidth ]{figures/fig_annotation_tool.PNG}
% \caption{The interface of the annotation tool that allows annotating the privacy policy document with 18 GDPR requirements.}
% \label{fig:annotation_tool}
% \end{figure}

% \end{appendices}
    
